# Supplementary material for: MultiOrg: A Multi-rater Organoid-detection Dataset
Source: arXiv:2410.14612 source file (2024-12-11)
Supplement: Supplementary file 2 [file fig_histogram_map_model_labels.tex]

\begin{figure}[h!!]
    \centering
    \includegraphics[width=0.6\textwidth]{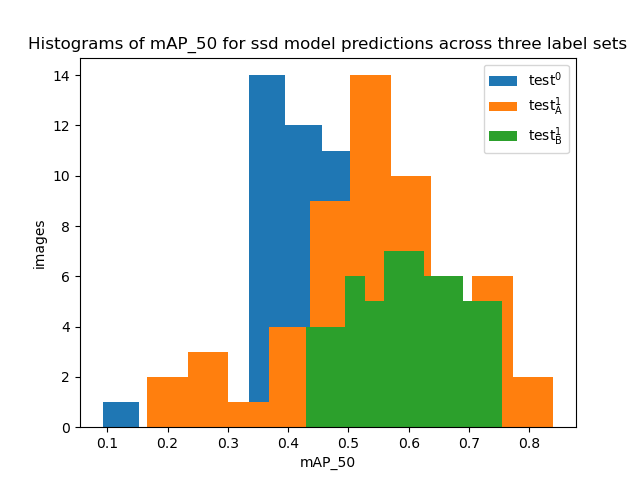}
    \caption{\eac{mAP} on the different label sets. Distributions of \eac{mAP} for the \eac{SSD} model predictions using the three label sets as \eac{GT}.
    The model is overall in more agreement with $test^1_A$ and $test^1_B$.
    We observe one outlier image in $test^0$ (\eac{mAP}<0.2).}
    \label{fig:hist-map}
\end{figure}
