# Supplementary material for: MultiOrg: A Multi-rater Organoid-detection Dataset
Source: arXiv:2410.14612 source file (2024-12-11)
Supplement: Supplementary file 3 [file fig_well_plate.tex]

\begin{figure}[ht]
    \centering
    \includegraphics[width=1.0\columnwidth]{96_well_plate.png}
    \caption{Biological experimental setup \& Image acquisition: An example of the \emph{Falcon®} 96-well Black/Clear Flat Bottom TC-treated Imaging Microplates. For each experiment in our setup, one such plate is used and images are acquired from all wells. The wells are then randomly sampled to comprise the 411 image samples of our dataset.}
    \label{fig:96_well_plate}
\end{figure}
